# Supplementary material for: Theme Enrichment Analysis: A Statistical Test for Identifying Significantly Enriched Themes in a List of Stories with an Application to the Star Trek Television Franchise
Source: arXiv:1707.06227 ancillary file (2018-08-14)
Supplement: Supplementary file 1 [file supplement.pdf]

# *Supplementary Material*: Theme Enrichment Analysis: A Statistical Test for Identifying Significantly Enriched Themes in a List of Stories with an Application to the Star Trek Television Franchise

## SUPPLEMENTARY NOTE 1

Star Trek has long been an important part of American popular culture [1], and remains popular among sci-fi enthusiasts the world over [2]. Those acquainted with the Star Trek science fiction media franchise will know that in the main it comprises seven television series and thirteen feature films [3]. Figure **??** shows an overview. The first series, which is known as *Star Trek: The Original Series* (or simply *TOS*), began airing in 1966 and ran for 80 mostly delightful episodes. It depicts the adventures of Captain James T. Kirk and his crew aboard the starship Enterprise on a five-year mission to explore the galaxy. The mission was temporarily suspended three years in when the show was cancelled in 1969 on account of poor ratings. But the Enterprise crew saw their mission through to completion in *Star Trek: The Animated Series* (*TAS*), which ran from 1973 to 1974 in two seasons consisting of 22 somewhat less delightful episodes. Six feature films following the TOS/TAS cast on subsequent adventures were released in the years from 1979 to 1991. From TOS was spawned the spin-off television series *Star Trek: The Next Generation* (*TNG*) which ran from 1987 to 1994 in seven seasons consisting of 178 episodes. It is set a generation or so after Captain Kirk's five-year mission. In the series, a fresh cast of characters is led by Captain Jean-Luc Picard on a similar mission of galactic exploration aboard a newfangled starship Enterprise. There are four associated feature films. Four subsequent television series have been produced: *Star Trek: Deep Space Nine* (1993 – 99), *Star Trek: Voyager* (1995 – 2001), and *Star Trek: Enterprise* (2001 – 05). Three reboot films based on TOS have also been released to date, and a seventh television series, *Star Trek: Discovery* (2017 – ), is presently being aired.

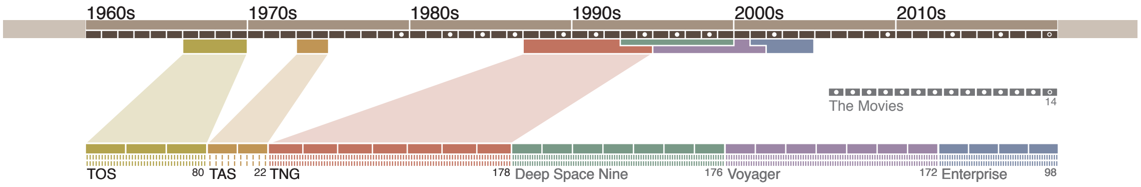


Figure S1: The Star Trek television series and film franchise overview.

[1] Hayes, N. (2016). Star Trek and the kiss that changed TV. URL: `http://www.bbc.com/culture/story/20160707-star-trek-turns-50-why-it-was-subversive-and-groundbreaking`. [Online; posted 7-July-2016]

[2] STARFLEET, the International Star Trek Fan Association, Inc. (2017). URL: `http://sfi.org/`. [Online; accessed 1-December-2017]

[3] Star Trek. (2017). URL: `http://www.startrek.com/`. [Online; accessed 1-December-2017]

## SUPPLEMENTARY NOTE 2

This supplementary note contains a description of the Klingon storyset from the case study of Subsection 4.1. The stories are summarized below in Table S1. The criteria for episode inclusion is simply that the aliens known as the Klingons are featured throughout the episode in a way that is central to the story.

**Table S1.** The Klingon storyset story IDs, titles, and brief episode summaries. Story ID format consists of a series identifier, followed by a season number, followed by an episode number.

| Story ID | Title | Summary |
|---|---|---|
| TOS1x27 | Errand of Mercy | The Enterprise is tasked to protect the Organians from Klingon aggression, but Kirk is left baffled when his offer of help is rejected. |
| TOS2x03 | Friday's Child | On a mission to secure a mining agreement on Capella IV, the Enterprise crew arrive to find that the Klingons have beaten them to the punch. |
| TOS2x13 | The Trouble with Tribbles | Tribbles disrupt a dispute between the Federation and the Klingon Empire over the ownership of a lucrative planet. |
| TOS2x16 | A Private Little War | Kirk must decide how to save a primitive race of hill-people from the technological interference of the Klingons. |
| TOS3x11 | Day of the Dove | An incorporeal alien that feeds on negative emotions drives the crew of the Enterprise into brutal conflict with the Klingons. |
| TOS3x22 | The Savage Curtain | Rock monsters force Kirk and Spock to team with Abraham Lincoln in an epic battle to the death against a team of legendary villains. |
| TAS1x05 | More Tribbles, More Troubles | The Enterprise crew become entangled in an ongoing conflict between the Klingons and the notorious tribble peddler Cyrano Jones. |
| TAS1x12 | The Time Trap | The Enterprise and a Klingon battlecruiser are drawn into a timeless dimension where fellow castaways from all the major alien races of the galaxy live together in peace. |
| TNG1x20 | Heart of Glory | A trio of Klingon fugitives seeking battle attempt to hijack the Enterprise, and ask Worf to join them. |
| TNG2x08 | A Matter Of Honor | Riker is assigned to a Klingon vessel via an officer exchange program between the Federation and the Klingon Empire. |
| TNG2x20 | The Emissary | Worf's old flame K'Ehleyr comes aboard Enterprise to help deal with a ship of Klingon sleeper agents unaware they are no longer at war. |
| TNG3x15 | Yesterday's Enterprise | The Enterprise-D's reality is altered into one where the Federation is in a desperate war with the Klingon Empire. |
| TNG3x17 | Sins of the Father | Worf stands trial to prove his father's innocence when the Klingon High Council accuses the family patriarch of treason. |
| TNG4x07 | Reunion | K'Ehleyr returns to the Enterprise to help mediate a Klingon power dispute and inform Worf that he has fathered her a son. |
| TNG4x21 | The Drumhead | An obsessed Starfleet admiral pursues a witch-hunt for suspected Romulan spies aboard the Enterprise. |
| TNG4x24 | The Mind's Eye | The Romulans condition Geordi to assassinate a Klingon governor. |
| TNG4x26 | Redemption | Worf leaves the Enterprise to fight in a brutal Klingon civil war. |
| TNG5x01 | Redemption II | The Federation ships intervenes in an ongoing Klingon civil war, resulting in Gowron's installation as Chancellor. |
| TNG5x16 | Ethics | When Worf is paralyzed in a freak accident, his sense of honor compels him to choose between between euthanasia and a risky medical procedure. |
| TNG6x13 | Aquiel | Geordi becomes infatuated with an alien Starfleet officer who is suspected of murdering her colleague while stationed at a far-flung space station. |
| TNG6x16 | Birthright, Part I | Worf is told on Deep Space Nine that his father is alive, and being held by the Romulans at a secret prison camp. |
| TNG6x17 | Birthright, Part II | When Worf is captured and taken to a Romulan operated Klingon refugee camp, he tries to teach the refugees the ways of the warrior. |
| TNG6x20 | The Chase | Picard tries to solve an ancient genetic mystery uncovered by his archaeological mentor, Richard Galen, but soon finds that the Klingons, Romulans, and Cardassians are already hot on the trail. |
| TNG6x22 | Suspicions | Beverly risks her career to vindicate a murdered Ferengi scientist in the eyes of his Klingon and Vulcan peers. |
| TNG6x23 | Rightful Heir | Worf experiences a crisis of faith, and travels to a Klingon holy site where the mythic figure Kahless returns to lead the Klingon people. |
| TNG7x21 | Firstborn | Worf and a mysterious family friend attempt to convince Worf's son Alexander to embrace his warrior heritage. |

## SUPPLEMENTARY NOTE 3

This supplementary note contains tables and a figure related to the comparison of the hypergeometric test with TF-IDF scoring as described in Section 4.4 of the main paper.

**Table S2.** TF-IDF scores for themes in Klingon-centric episodes relative to *TOS*/*TAS* and *TNG* backgrounds, respectively.

| Rank | Theme | Domain | $k/K$ | TF-IDF |
|---|---|---|---|---|
| | Top 20 Enriched Themes in *TOS*/*TAS* Klingon Episodes | | | |
| 1 | über-belligerent alien | 🟡 | 5/5 | 1.88 |
| 2 | diplomatic negotiating | 🟢 | 4/7 | 1.34 |
| 3 | culturally distinguished life form | 🟡 | 6/20 | 1.22 |
| 4 | man vs. beast | 🔴 | 3/5 | 1.13 |
| 5 | diplomacy | 🟢 | 5/19 | 1.05 |
| 6 | pacifism | 🔴 | 3/7 | 1.00 |
| 7 | military tactics | 🔵 | 3/7 | 1.00 |
| 8 | conflict over a shared resource | 🟢 | 2/2 | 0.98 |
| 9 | atrocities of war | 🟢 | 2/2 | 0.98 |
| 10 | tribble | 🟡 | 2/2 | 0.98 |
| 11 | war | 🟢 | 5/22 | 0.96 |
| 12 | miscellaneous life form | 🟡 | 3/8 | 0.95 |
| 13 | imperialistic society | 🟢 | 3/8 | 0.95 |
| 14 | the art of war | 🔵 | 5/23 | 0.93 |
| 15 | cross cultural understanding | 🟢 | 4/16 | 0.93 |
| 16 | humility | 🔴 | 3/9 | 0.91 |
| 17 | conflict of moral codes | 🟢 | 2/3 | 0.88 |
| 18 | patience | 🔴 | 3/10 | 0.87 |
| 19 | transnational social issue | 🟢 | 6/32 | 0.87 |
| 20 | temperance | 🔴 | 2/4 | 0.81 |
| | Top 20 Enriched Themes in *TNG* Klingon Episodes | | | |
| 1 | über-belligerent alien | 🟡 | 14/14 | 1.97 |
| 2 | honor | 🔴 | 13/18 | 1.65 |
| 3 | culturally distinguished life form | 🟡 | 14/53 | 0.93 |
| 4 | the need for cultural heritage | 🔴 | 5/8 | 0.86 |
| 5 | rage | 🔴 | 7/23 | 0.79 |
| 6 | belonging | 🔴 | 7/27 | 0.73 |
| 7 | father and son | 🔴 | 6/21 | 0.71 |
| 8 | the art of war | 🔵 | 6/24 | 0.66 |
| 9 | loyalty | 🔴 | 7/33 | 0.65 |
| 10 | surprise | 🔴 | 6/27 | 0.62 |
| 11 | wrath | 🔴 | 8/44 | 0.62 |
| 12 | guilt and evidence | 🟢 | 4/11 | 0.62 |
| 13 | cooperation | 🔴 | 5/20 | 0.60 |
| 14 | diligence | 🔴 | 7/38 | 0.60 |
| 15 | racism in society | 🟢 | 3/5 | 0.59 |
| 16 | facing wrongful accusations | 🔴 | 3/5 | 0.59 |
| 17 | human need | 🔴 | 9/54 | 0.59 |
| 18 | disgust | 🔴 | 5/22 | 0.58 |
| 19 | personal conviction | 🔴 | 5/23 | 0.57 |
| 20 | the lust for power | 🔴 | 3/7 | 0.54 |

**Table S3.** TF-IDF scores for themes in each Star Trek television series relative to a *TOS*/*TAS*/*TNG* background.

| Rank | Theme | Domain | $k/K$ | TF-IDF |
|---|---|---|---|---|
| | **Top 20 TOS Enriched Themes** | | | |
| 1 | wrath | 🔴 | 41/85 | 0.61 |
| 2 | gender issues | 🟢 | 26/46 | 0.58 |
| 3 | female stereotype | 🟢 | 19/24 | 0.58 |
| 4 | rage | 🔴 | 27/50 | 0.58 |
| 5 | alternate society | 🟡 | 45/100 | 0.58 |
| 6 | alternate life | 🟡 | 39/87 | 0.57 |
| 7 | existential risk | 🟡 | 37/83 | 0.56 |
| 8 | what if I faced an incredible situation | 🟡 | 30/64 | 0.55 |
| 9 | way of life | 🔴 | 24/45 | 0.55 |
| 10 | past and present moral controversies | 🟢 | 24/49 | 0.52 |
| 11 | man-made existential risk | 🟡 | 22/43 | 0.51 |
| 12 | ethics | 🔵 | 31/74 | 0.51 |
| 13 | personal ethical dilemma | 🔴 | 45/112 | 0.51 |
| 14 | serenity | 🔴 | 21/41 | 0.50 |
| 15 | disagreeable characteristic | 🔴 | 48/121 | 0.50 |
| 16 | social order | 🟢 | 22/48 | 0.48 |
| 17 | lust | 🔴 | 28/70 | 0.48 |
| 18 | compassion | 🔴 | 25/60 | 0.48 |
| 19 | personal practical dilemma | 🔴 | 26/64 | 0.48 |
| 20 | amicable disposition | 🔴 | 45/119 | 0.48 |
| | **Top 10 TAS Enriched Themes** | | | |
| 1 | earth-life inspired life form | 🟡 | 6/15 | 0.80 |
| 2 | miscellaneous life form | 🟡 | 5/13 | 0.70 |
| 3 | life-support belt | 🟡 | 3/3 | 0.62 |
| 4 | what if my life were different | 🟡 | 6/38 | 0.54 |
| 5 | alternate society | 🟡 | 11/100 | 0.51 |
| 6 | crackpot theory | 🔵 | 5/30 | 0.51 |
| 7 | existential risk | 🟡 | 9/83 | 0.49 |
| 8 | man vs. beast | 🔴 | 3/8 | 0.48 |
| 9 | alternate life | 🟡 | 9/87 | 0.48 |
| 10 | what's out there | 🟡 | 6/51 | 0.46 |
| | **Top 20 TNG Enriched Themes** | | | |
| 1 | familial love | 🔴 | 49/59 | 0.43 |
| 2 | pride | 🔴 | 51/64 | 0.43 |
| 3 | familial relations | 🔴 | 81/111 | 0.42 |
| 4 | family affairs | 🔴 | 91/126 | 0.41 |
| 5 | growing up | 🔴 | 40/47 | 0.40 |
| 6 | culturally distinguished life form | 🟡 | 53/73 | 0.40 |
| 7 | group interaction | 🔴 | 66/96 | 0.40 |
| 8 | heavenly virtue | 🔴 | 105/144 | 0.39 |
| 9 | human nature | 🔵 | 57/83 | 0.39 |
| 10 | AI technology | 🟡 | 45/61 | 0.39 |
| 11 | state of mind | 🔴 | 81/120 | 0.39 |
| 12 | views and customs | 🟢 | 88/129 | 0.38 |
| 13 | fictional apparatus | 🟡 | 54/80 | 0.38 |
| 14 | annoyance | 🔴 | 56/84 | 0.38 |
| 15 | virtual reality room | 🟡 | 31/32 | 0.38 |
| 16 | introspection | 🔴 | 106/149 | 0.38 |
| 17 | android | 🟡 | 33/38 | 0.37 |
| 18 | coping with an affliction | 🔴 | 46/67 | 0.37 |
| 19 | agreeable characteristic | 🔴 | 96/142 | 0.37 |
| 20 | intercultural relations | 🟢 | 95/141 | 0.37 |

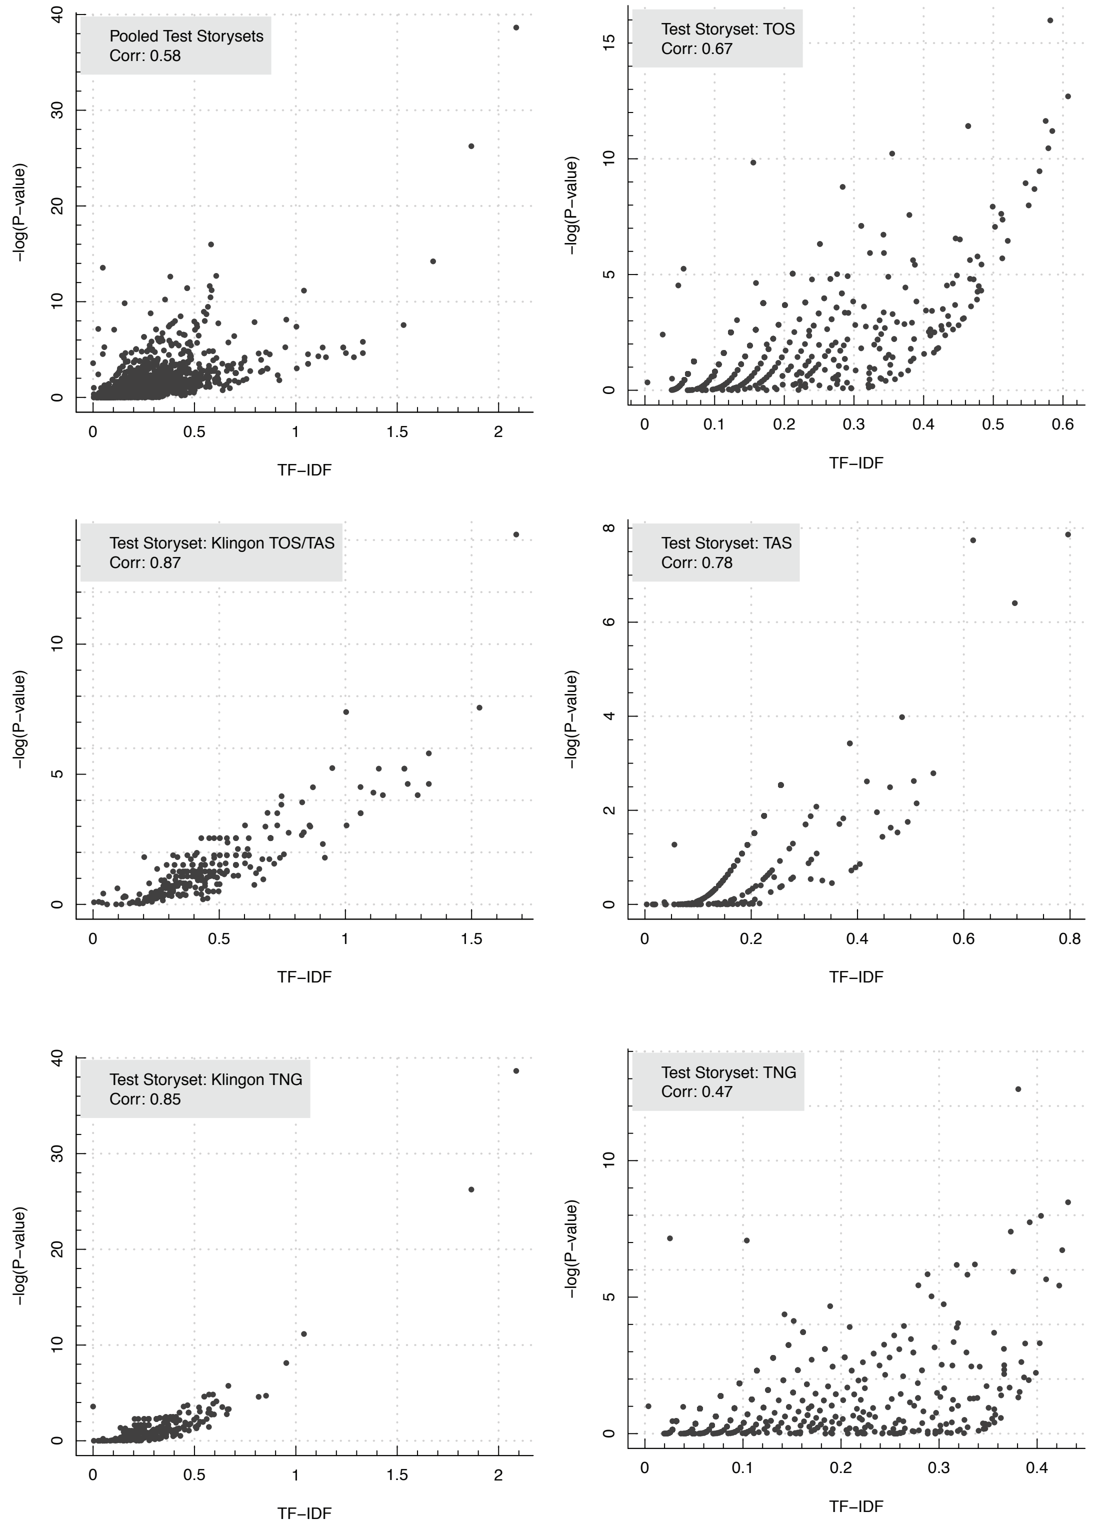


Figure S2: Scatterplots of TF-IDF scores versus hypergeometric test negative logarithm *p*-values for themes from each enrichment analysis from Sections 4.1 and 4.2 of the main text. The upper left scatterplot shows the pooled results from all five cases.
